# Supplementary material for: MedAide: Information Fusion and Anatomy of Medical Intents via LLM-based Agent Collaboration
Source: arXiv:2410.12532 source file (2025-07-03)
Supplement: Supplementary file 1 [file appendix.tex]

\section{Appendix}
\subsection{Secondary Level Headings}
\subsubsection{Three Level Headings}
\vspace{0.3pt}\noindent\textbf{Fourth Level Headings}\hspace{1ex}
This is used to test the format of the content.
